# Supplementary material for: One-Dimensional Edge States with Giant Spin Splitting in a Bismuth Thin Film
Source: arXiv:1502.03197 source file (2015-02-11)
Supplement: Supplementary file 1 [file Takayama-SM.pdf]

# One-Dimensional Edge States with Giant Spin Splitting in a Bismuth Thin Film

### Supplemental Material

## 1. Relationship between three edge domains and electronic states

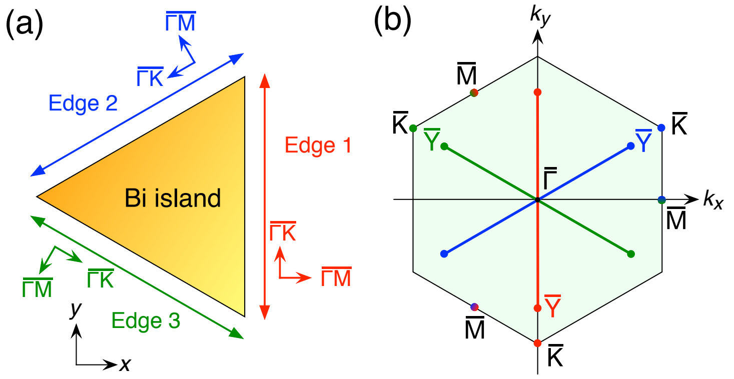


**FIG. S1.** Relationship between edge domains in real space and high-symmetry lines in $k$ space. (a) Schematic illustration of three different edges (edge 1-3) at triangular-shaped 1BL Bi island. (b) The $\bar{\Gamma}$- $\bar{\mathrm{Y}}$ cut (same as the $\bar{\Gamma}$- $\bar{\mathrm{K}}$ cut) for each edge in the hexagonal surface Brillouin zone. Common colorings (blue, red, and green) are used to specify the contribution from each edge.

As schematically shown in Fig. S1(a), triangular-shaped islands are formed on the top of the Bi thin film as also visible in the atomic-force-microscopy image of Fig. 3(a), wherein three different edges rotated by 120° from each other (for convenience, we label them as edge 1-3) are inherently involved. When we assume only the edge-1 structure running along the $y$ direction, no dispersion is expected along the $k_x$ direction (the $\bar{\Gamma}$- $\bar{\mathrm{M}}$ direction) due to its 1D nature. However, the mixture of three edge domains is expected to equally contribute to the observed electronic states in the ARPES data, indicating that the faint dispersive features observed along the $k_x$ cut in Fig. 1(c) do not originate from edge 1, but from edges 2 and 3 where the angle between edge direction and $k_x$ axis is 30° as shown in Fig. S1(b). Despite such a complication, we can safely conclude the 1D nature of the edge state due to the fact that the observed dispersive near-$E_F$ feature around the $\bar{\mathrm{Y}}$ point purely originate from a single edge; namely, the energy location of bands for two other edges are away from $E_F$ around the $\bar{\mathrm{Y}}$ point.

## 2. Edge band dispersion around the $\overline{\mathrm{M}}$ point

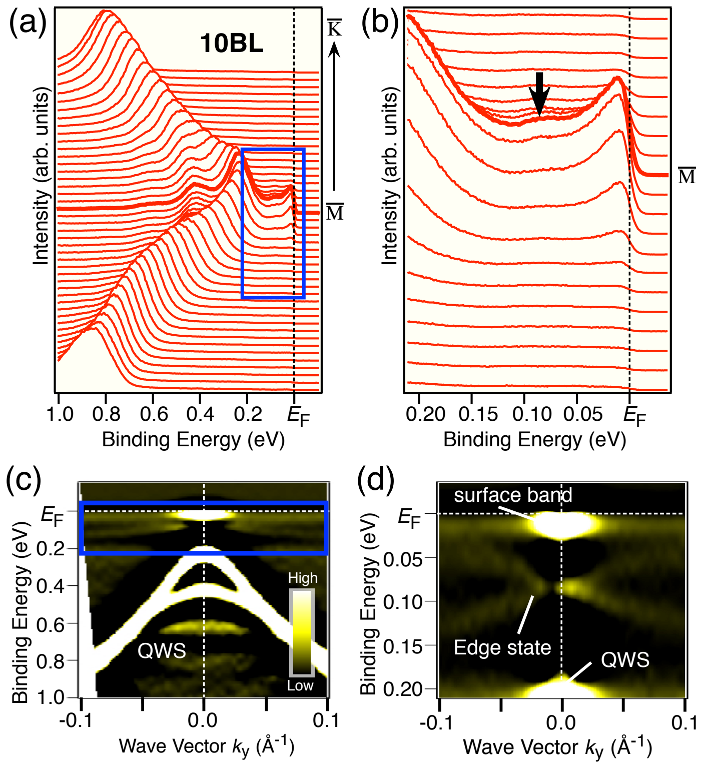


**FIG. S2.** Edge state of Bi around the $\overline{\mathrm{M}}$ point. (a) ARPES spectra of Bi thin film ($d$ = 10BL) measured along the $\overline{\mathrm{M}}$- $\overline{\mathrm{K}}$ cut. (b) Same as (a) but magnified in the vicinity of $E_F$ as shown by blue rectangle in (a). (c), (d) Second-derivative plot of the ARPES intensity for (a) and (b), respectively.

As shown in the energy distribution curves (EDCs) and the intensity plot of Bi thin film ($d$ = 10BL) in Figs. S2(a) and S2(c), the experimental band dispersion along the $\overline{\mathrm{M}}$- $\overline{\mathrm{K}}$ cut shows multiple holelike bands originating from the quantum well states (QWS). Top of the QWS is located at ~ 0.2 eV binding energy below $E_F$. We also find a shallow electronlike surface state in the close vicinity of $E_F$ centered at the $\overline{\mathrm{M}}$ point which is separated from the QWS *via* the band gap situated at $E_F$ - 0.2 eV. As clearly visible from the magnified EDCs in Fig. S2(b), we find a weak signature of a hump at ~ 75 meV inside the band gap (see arrow). As seen in Fig. S2(d), the hump shows a characteristic "$x$"-shaped energy dispersion whose intersection is located at the $\overline{\mathrm{M}}$ point, similarly to the case of edge band dispersion along the $\overline{\Gamma}$- $\overline{\mathrm{Y}}$ direction [see Fig. 2(c)]. This is reasonable since the $\overline{\mathrm{M}}$ point is the horizontal projection of the $\overline{\mathrm{Y}}$ point for

simulated crystal structure [see also Fig. 3(b)]. In fact, the estimated energy position of the Kramers point at the $\bar{\mathrm{M}}$ point coincides well with that at the $\bar{\mathrm{Y}}$ point within our experimental uncertainty, supporting this assignment. It is also suggested from the argument in section 1 that the *x*-shaped dispersion along the $\bar{\mathrm{M}}$- $\bar{\mathrm{K}}$ cut does not arise from the edge parallel to the $\bar{\mathrm{M}}$- $\bar{\mathrm{K}}$ direction but originates from two other edges [In Fig. S1 case; when the $\bar{\mathrm{M}}$- $\bar{\mathrm{K}}$ direction is parallel to the edge-1 direction (*y* axis), the *x*-shaped band originates from edges 2 and 3].

### 3. Thickness dependence of the edge state

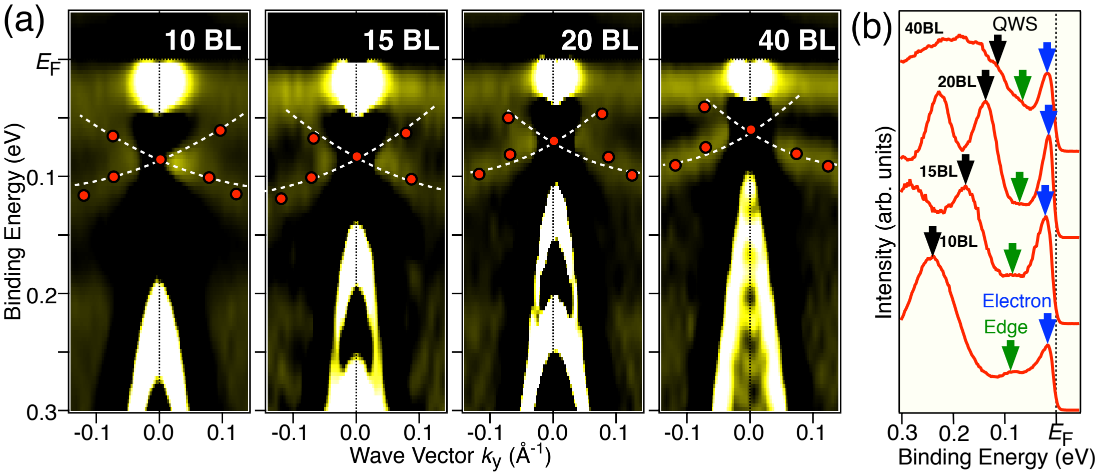


**FIG. S3.** Thickness-dependence of the band dispersion. (a) Second-derivative plots of the near-$E_F$ ARPES intensity along the $\bar{\mathrm{M}}$- $\bar{\mathrm{K}}$ cut for various film thickness ($d$ = 10, 15, 20, and 40 BL). Energy position of the edge bands are shown by red dots. Dashed lines are guides for eyes to trace the edge band dispersion. (b) Thickness dependence of the EDC at the $\bar{\mathrm{M}}$ point. Black, green, and blue arrows represent the top of the QWS, the edge band, and the bottom of the electronlike surface band, respectively.

To elucidate the nature of the edge band in more detail, we have performed ARPES measurements for various film thickness *d*. We have chosen the $\bar{\mathrm{M}}$ point for this study to accurately estimate the film thickness from the energy location of the QWS. The experimental band dispersion for $d$ = 10-40 BL is displayed in Fig. S3(a). One can immediately notice that the *x*-shaped edge band always appears irrespective of the film thickness. Moreover, its energy location is robust to the variation in the film thickness, in contrast to the marked energy shift of the QWS. This is reasonable since Bi islands

which contain edge structure would always remain on the surface regardless of the film thickness. The energy position of the Kramers point appears to show a slight thickness-dependence as recognized in EDCs in Fig. S3(b), probably due to a small difference in the carrier concentration of the edge and/or the finite interactions between topmost Bi bilayer island and the Bi film beneath it.

### 4. Aging effect of the edge state

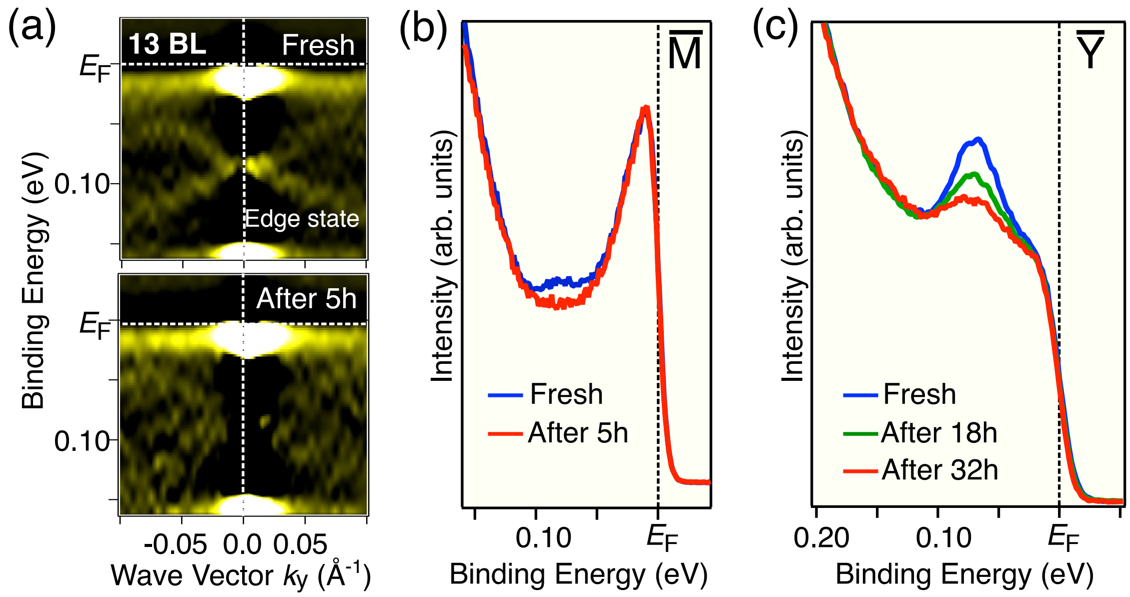


**FIG. S4.** Aging effect of the edge state. (a) Second-derivative plot of the ARPES intensity along the $\bar{M}$- $\bar{K}$ cut for $d$ = 13BL for two samples just after preparation (top) and 5 hours after it (bottom). (b), (c) Aging effect of EDC at the $\bar{M}$ and $\bar{Y}$ points, respectively.

Figure S4 shows the aging effect of the edge band intensity for $d$ = 13BL. As seen in Fig. S4(a), we observe the $x$-shaped dispersion for the sample just after preparation, while the $x$-shaped band almost vanishes after five hours. As also visible in Figs. S4(b) and (c) which directly show time evolution of the EDC at the $\bar{M}$ point and the $\bar{Y}$ point, respectively, the peak feature seen in the fresh surface gradually reduces its weight, whereas the surface band and the QWS do not show meaningful time evolution in a period of a few days. This result demonstrates that the edge band is sensitive to the surface aging. We speculate that the dangling bonds of the edge state were gradually

passivated after the sample growth, by residual gases, while the source of gases is unknown (probably, hydrogen, water, carbon oxides, *etc*.). The 2D surface states and QWS were found to be robust against such gas absorption, likely due to the absence of dangling bonds. We note that all the ARPES measurements presented in Figs. 1-3 have been obtained within a few hours after the sample preparation to avoid aging effect for the edge state.

**5. Calculations for two types of edge structures**

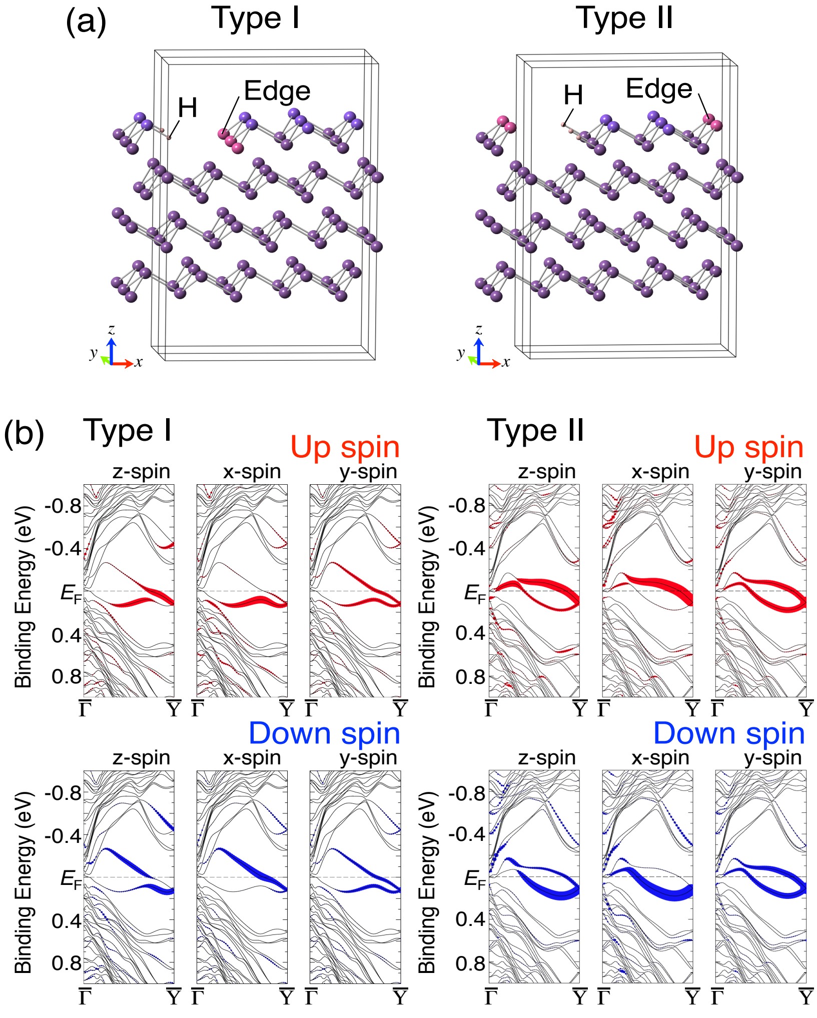


**FIG. S5.** Band calculations for two types of edge structures. (a) Two types of edge structures (type I and II), in which the band calculations have been carried out. (b) Calculated band dispersions along the $\bar{\Gamma}$- $\bar{Y}$ line for type I (left) and type II (right) edge structure. The thickness of red or blue curves indicates the concentration of the up- and down-spin electrons along the axis specified in the figure.

Bi islands were modeled by a 1-BL thick ribbon structure on the Bi slab. There are two types of edge structures for the Bi ribbon. As shown in Fig. S5(a), Bi atoms at the second layer form the edge structure for type-I case, whereas the topmost layer forms the type-II edge structure. The other side of the edge was terminated by hydrogen atoms. In either case, the calculated bands clearly show a Rashba splitting as seen in Fig. S5(b). We found that the calculated edge band structure for type II shows a better agreement with our ARPES experiment, though type I edge is slightly more stable than type II. Figure S5(b) shows the band structure with projection of the wave functions on the edge Bi spin. Calculated spin polarization has a sizable out-of-plane $z$ component besides the in-plane $x$ component, unlike the case of ideal 2D Rashba states which only contains the in-plane component. The finite $z$ component is related to the structure of the edge which breaks the space-inversion symmetry for the $x$-direction, and the finite $z$-spin polarization is experimentally confirmed by the spin-resolved ARPES measurement as shown in Fig. 3(f).
